# Supplementary material for: Quantifying an Interference-Assisted Signal Strength Breathing Surveillance Attack
Source: arXiv:1905.03939 source file (2019-05-10)
Supplement: Supplementary file 1 [file appendix.tex]

%%%%%%%%%%%%%%%%%%%%%%
\section*{Appendix A}
\label{app:partial}

\subsection*{Proof for Partial Derivatives}
Given ${\cal C}_k \coloneqq \cos (\omega T_s k+\phi)$, ${\cal S}_k \coloneqq \sin (\omega T_s k+\phi)$ and $q\in\{-1, +1\}$, then

% wrt A
\begin{equation}
\begin{aligned}
\dfrac{\partial}{\partial A} f_{y[k]}(q;{\bm \theta})&= \frac{1}{2}\dfrac{\partial}{\partial A} {\rm erfc}\left(-\dfrac{q}{\sqrt{2}\sigma}(A{\cal C}_k +B)\right)\\
&= \frac{1}{\sqrt{\pi}} \exp{\left(-\frac{1}{2\sigma^2}\left(A{\cal C}_k+B\right)^2\right)}\dfrac{\partial}{\partial A}\left(-\dfrac{q}{\sqrt{2}\sigma}(A{\cal C}_k +B)\right)\\
&= -\frac{q{\cal C}_k}{\sqrt{2\pi} \sigma} \exp{\left(-\frac{1}{2\sigma^2}\left(A{\cal C}_k+B\right)^2\right)}
\end{aligned}
\end{equation}

% wrt B
\begin{equation}
\begin{aligned}
\dfrac{\partial}{\partial B} f_{y[k]}(q;{\bm \theta})&= \frac{1}{2}\dfrac{\partial}{\partial B} {\rm erfc}\left(-\dfrac{q}{\sqrt{2}\sigma}(A{\cal C}_k +B)\right)\\
&= \frac{1}{\sqrt{\pi}} \exp{\left(-\frac{1}{2\sigma^2}\left(A{\cal C}_k+B\right)^2\right)}\dfrac{\partial}{\partial B}\left(-\dfrac{q}{\sqrt{2}\sigma}(A{\cal C}_k +B)\right)\\
&= -\frac{q}{\sqrt{2 \pi} \sigma} \exp{\left(-\frac{1}{2\sigma^2}\left(A{\cal C}_k+B\right)^2\right)}
\end{aligned}
\end{equation}

% wrt \omega
\begin{equation}
\begin{aligned}
\dfrac{\partial}{\partial \omega} f_{y[k]}(q;{\bm \theta})&= \frac{1}{2}\dfrac{\partial}{\partial \omega} {\rm erfc}\left(-\dfrac{q}{\sqrt{2}\sigma}(A{\cal C}_k +B)\right)\\
&= \frac{1}{\sqrt{\pi}} \exp{\left(-\frac{1}{2\sigma^2}\left(A{\cal C}_k+B\right)^2\right)}\dfrac{\partial}{\partial \omega}\left(-\dfrac{q}{\sqrt{2\sigma}}(A{\cal C}_k +B)\right)\\
&= \frac{qAT_sk{\cal S}_k}{\sqrt{2\pi} \sigma} \exp{\left(-\frac{1}{2\sigma^2}\left(A{\cal C}_k+B\right)^2\right)}
\end{aligned}
\end{equation}

% wrt phi
\begin{equation}
\begin{aligned}
\dfrac{\partial}{\partial \phi} f_{y[k]}(q;{\bm \theta})&= \frac{1}{2}\dfrac{\partial}{\partial \phi} {\rm erfc}\left(-\dfrac{q}{\sqrt{2}\sigma}(A{\cal C}_k +B)\right)\\
&= \frac{1}{\sqrt{\pi}} \exp{\left(-\frac{1}{2\sigma^2}\left(A{\cal C}_k+B\right)^2\right)}\dfrac{\partial}{\partial \phi}\left(-\dfrac{q}{\sqrt{2}\sigma}(A{\cal C}_k +B)\right)\\
&= \frac{qA{\cal S}_k}{\sqrt{2\pi} \sigma} \exp{\left(-\frac{1}{2\sigma^2}\left(A{\cal C}_k+B\right)^2\right)}
\end{aligned}
\end{equation}
%%%%%%%%%%%%%%%%%%%%%%%%
\fi
